# Supplementary material for: Unsupervised Question Decomposition for Question Answering
Source: arXiv:2002.09758 source file (2020-10-06)
Supplement: Supplementary file 1 [file decomps_in_appendix.tex]

\begin{table*}[th!]
    \centering
    \scriptsize
    % \scalebox{0.9}{
    \begin{tabular}{p{1.2cm}p{15cm}}
            \toprule

    \multicolumn{2}{c}{  {\bf Q:} What is the name of the singer who's song was released as the lead single from the album "Confessions", and that had popular song stuck behind for eight consecutive weeks?} \\ \midrule \multirow{2}{1cm}{\useqtoseq + Random}
            & {\bf Sub-Q1} what is the name of the singer who 's song was released as the lead single from the album " confessions? \\
             %& {\bf Sub-A1} is a song by American singer Usher. He co-wrote the song with Sean Garrett, Patrick J. Que Smith, Robert McDowell, LRoc, Ludacris, Da'Ron, and Lil Jon. \\
            &  {\bf Sub-Q2}  why did popular song stuck behind for eight consecutive weeks? \\
            %& {\bf Sub-A2} It reached number 1 in the United Kingdom and in Netherlands, and number 2 in the United States, stuck for eight consecutive weeks behind the Usher singles "Yeah" and "Burn", respectively. \\
            \cmidrule(l){1-2}
  \multirow{2}{1cm}{\useqtoseq + FastText}
                 & {\bf Sub-Q1} what is the name of the singer? \\
                 %& {\bf Sub-A1} "No One" is a song by American singer and songwriter Alicia Keys from her third studio album, "As I Am" (2007). \\
                &   {\bf Sub-Q2}  what song was released as the lead single from the album " confessions , " and that had popular song stuck behind for eight consecutive weeks? \\
            %& {\bf Sub-A2} "Yeah!" is a song by American singer Usher. \\
                \cmidrule(l){1-2}
  \multirow{2}{1cm}{\seqtoseq + Random}
                 & {\bf Sub-Q1} what is the maximum number of students allowed to take part in the program? \\
                 %& {\bf Sub-A1} "No One" is a song by American singer and songwriter Alicia Keys from her third studio album, "As I Am" (2007). \\
                &   {\bf Sub-Q2}  what is the maximum number of students allowed per year? \\
            %& {\bf Sub-A2} "No One" is a song by American singer and songwriter Alicia Keys from her third studio album, "As I Am" (2007). \\
                \cmidrule(l){1-2}
  \multirow{2}{1cm}{\seqtoseq + FastText}
                 & {\bf Sub-Q1} what is the name of the lead singer of the group? \\
                 %& {\bf Sub-A1} Billy Ray Cyrus is an American country music singer, songwriter, actor and philanthropist, who helped make country music a worldwide phenomenon. \\
                &   {\bf Sub-Q2}  when was the last time you heard a song called " on and on " by a female vocalist? \\
            %& {\bf Sub-A2} "No One" is a song by American singer and songwriter Alicia Keys from her third studio album, "As I Am" (2007). It was written and produced by Keys, Kerry Brothers Jr., and George M. Harry, and released as the album's lead single on September 11, 2007. \\
                \cmidrule(l){1-2}
  \multirow{2}{1cm}{PseudoD + Random}
                 & {\bf Sub-Q1} what was sold to foreign ptts? \\
                 %& {\bf Sub-A1} "No One" is a song by American singer and songwriter Alicia Keys from her third studio album, "As I Am" (2007). \\
                &   {\bf Sub-Q2}  what tends to lead to less money? \\
            %& {\bf Sub-A2} "No One" is a song by American singer and songwriter Alicia Keys from her third studio album, "As I Am" (2007). \\
                \cmidrule(l){1-2}
  \multirow{2}{1cm}{PseudoD + FastText}
                 & {\bf Sub-Q1} which single was released as the album 's lead single? \\
                 %& {\bf Sub-A1} "No One" is a song by American singer and songwriter Alicia Keys from her third studio album, "As I Am" (2007). \\
                &   {\bf Sub-Q2}  who did the song writing , what are some of the stories behind the songs? \\
            %& {\bf Sub-A2} It was written and produced by Keys, Kerry Brothers Jr., and George M. Harry, and released as the album's lead single on September 11, 2007. \\
                \cmidrule(l){1-2}
  \multirow{2}{1cm}{DecompRC}
                 & {\bf Sub-Q1} which singer? \\
                 %& {\bf Sub-A1} "No One" is a song by American singer and songwriter Alicia Keys from her third studio album, "As I Am" (2007). \\
                &   {\bf Sub-Q2}  what is the name of alicia keys 's song was released as the lead single from the album "confessions", and that had popular song stuck behind for eight consecutive weeks? \\
            %& {\bf Sub-A2} It reached number 1 in the United Kingdom and in Netherlands, and number 2 in the United States, stuck for eight consecutive weeks behind the Usher singles "Yeah" and "Burn", respectively. \\
                \cmidrule(l){1-2}
  \multirow{3}{1cm}{Variable \useqtoseq + FastText}
            & {\bf Sub-Q1} what is the name of the singer? \\
            % &  {\bf Sub-A1} is a song by american singer usher. he co-wrote the song with sean garrett, patrick j. que smith, robert mcdowell, lroc, ludacris, da'ron, and lil jon. \\
            & {\bf Sub-Q2}  who ' s the song was released as the lead single from the album? \\
            %& {\bf Sub-A2} "no one" is a song by american singer and songwriter alicia keys from her third studio album, "as i am" (2007). \\&
            & {\bf Sub-Q3}  what popular song was stuck behind for eight consecutive weeks? \\
            % & {\bf Sub-A3}  it reached number 1 in the united kingdom and in netherlands, and number 2 in the united states, stuck for eight consecutive weeks behind the usher singles "yeah" and "burn", respectively. \\
        \bottomrule
    \end{tabular}
    % }
    \vskip -0.7em
    \caption{Various decomposition methods for the question ``What is the name of the singer who's song was released as the lead single from the album ``Confessions,'' and that had popular song stuck behind for eight consecutive weeks?" Here, the Variable \useqtoseq{} model decomposed the question into three subquestions rather than two.}
    \label{tab:appendix_decomp_examples_3}
    \end{table*}     

\begin{table*}[th!]
    \centering
    \scriptsize
    % \scalebox{0.9}{
    \begin{tabular}{p{1.2cm}p{15cm}}
        \toprule
\multicolumn{2}{c}{  {\bf Q:} Are both Coldplay and Pierre Bouvier from the same country?} \\ \midrule \multirow{2}{1cm}{\useqtoseq + Random}
            & {\bf Sub-Q1} why are both coldplay and pierre bouvier from the same country? \\
             %& {\bf Sub-A1} Coldplay are a British rock band formed in 1996 by lead vocalist and keyboardist Chris Martin and lead guitarist Jonny Buckland at University College London (UCL). \\
            &  {\bf Sub-Q2}  what is the purpose of a speech? \\
            %& {\bf Sub-A2} Pierre Charles Bouvier (born 9 May 1979) is a Canadian singer, songwriter, musician, composer and actor who is best known as the lead singer and guitarist of the rock band Simple Plan. \\
            \cmidrule(l){1-2}
  \multirow{2}{1cm}{\useqtoseq + FastText}
                 & {\bf Sub-Q1} where are coldplay and coldplay from? \\
                 %& {\bf Sub-A1} Coldplay are a British rock band formed in 1996 by lead vocalist and keyboardist Chris Martin and lead guitarist Jonny Buckland at University College London (UCL). \\
                &   {\bf Sub-Q2}  what country is pierre bouvier from? \\
            %& {\bf Sub-A2} Pierre Charles Bouvier  (born 9 May 1979) is a Canadian singer, songwriter, musician, composer and actor who is best known as the lead singer and guitarist of the rock band Simple Plan. \\
                \cmidrule(l){1-2}
  \multirow{2}{1cm}{\seqtoseq + Random}
                 & {\bf Sub-Q1} what is the maximum number of students allowed to take part in the program? \\
                 %& {\bf Sub-A1} Coldplay are a British rock band formed in 1996 by lead vocalist and keyboardist Chris Martin and lead guitarist Jonny Buckland at University College London (UCL). \\
                &   {\bf Sub-Q2}  what is the maximum number of students allowed to take part in the course of the course of the course of the course of the course of the course of the course of the course of the course of the course of the course of the course of the course of the course of? \\
            %& {\bf Sub-A2} Coldplay are a British rock band formed in 1996 by lead vocalist and keyboardist Chris Martin and lead guitarist Jonny Buckland at University College London (UCL). \\
                \cmidrule(l){1-2}
  \multirow{2}{1cm}{\seqtoseq + FastText}
                 & {\bf Sub-Q1} who are similar musical artists to pierre bouvier? \\
                 %& {\bf Sub-A1} Coldplay are a British rock band formed in 1996 by lead vocalist and keyboardist Chris Martin and lead guitarist Jonny Buckland at University College London (UCL). \\
                &   {\bf Sub-Q2}  in the same year , pierre bouvier , pierre bouvier , pierre bouvier and pierre bouvier? \\
            %& {\bf Sub-A2} Pierre Charles Bouvier  (born 9 May 1979) is a Canadian singer, songwriter, musician, composer and actor who is best known as the lead singer and guitarist of the rock band Simple Plan. \\
                \cmidrule(l){1-2}
  \multirow{2}{1cm}{PseudoD + Random}
                 & {\bf Sub-Q1} in what year did fermat declare fermat 's little theorem? \\
                 %& {\bf Sub-A1} Coldplay are a British rock band formed in 1996 by lead vocalist and keyboardist Chris Martin and lead guitarist Jonny Buckland at University College London (UCL). \\
                &   {\bf Sub-Q2}  when did the united states withdraw from the bretton woods accord? \\
            %& {\bf Sub-A2} It first aired on MTV on March 6, 2005. The last episode was broadcast on April 24, 2005. \\
                \cmidrule(l){1-2}
  \multirow{2}{1cm}{PseudoD + FastText}
                 & {\bf Sub-Q1} what do a handful of couples have in common with coldplay , coldplay , and pierre bouvier? \\
                 %& {\bf Sub-A1} Coldplay are a British rock band formed in 1996 by lead vocalist and keyboardist Chris Martin and lead guitarist Jonny Buckland at University College London (UCL). \\
                &   {\bf Sub-Q2}  where are the french alps? \\
            %& {\bf Sub-A2} St Pierre is a former parish and hamlet in Monmouthshire, south east Wales, 3 mi south west of Chepstow and adjacent to the Severn estuary. \\
                \cmidrule(l){1-2}
  \multirow{2}{1cm}{DecompRC}
                 & {\bf Sub-Q1} is coldplay from which country? \\
                 %& {\bf Sub-A1} Coldplay are a British rock band formed in 1996 by lead vocalist and keyboardist Chris Martin and lead guitarist Jonny Buckland at University College London (UCL). \\
                &   {\bf Sub-Q2}  is pierre bouvier from which country? \\
            %& {\bf Sub-A2} Pierre Charles Bouvier (born 9 May 1979) is a Canadian singer, songwriter, musician, composer and actor who is best known as the lead singer and guitarist of the rock band Simple Plan. \\
                \cmidrule(l){1-2}
  \multirow{2}{1cm}{Variable \useqtoseq + FastText}
            & {\bf Sub-Q1} who are similar musical artists to coldplay? \\
            % &  {\bf Sub-A1} pierre charles bouvier (born 9 may 1979) is a canadian singer, songwriter, musician, composer and actor who is best known as the lead singer and guitarist of the rock band simple plan. \\
            &  {\bf Sub-Q2}  where is pierre bouvier from? \\
            %& {\bf Sub-A2} pierre charles bouvier  (born 9 may 1979) is a canadian singer, songwriter, musician, composer and actor who is best known as the lead singer and guitarist of the rock band simple plan. \\
        \bottomrule
    \end{tabular}
    % }
    \vskip -0.7em
    \caption{Various decomposition methods for the question ``Are both Coldplay and Pierre Bouvier from the same country?"}
    \label{tab:appendix_decomp_examples_1}
    \end{table*}

            \begin{table*}[th!]
    \centering
    \scriptsize
    % \scalebox{0.9}{
    \begin{tabular}{p{1.2cm}p{15cm}}
            \toprule

\multicolumn{2}{c}{  {\bf Q:} Who is older, Annie Morton or Terry Richardson?} \\ \midrule \multirow{2}{1cm}{\useqtoseq + Random}
            & {\bf Sub-Q1} who is older , annie morton? \\
             %& {\bf Sub-A1} Annie Morton (born October 8, 1970) is an American model born in Pennsylvania. \\
            &  {\bf Sub-Q2}  who is terry richardson? \\
            %& {\bf Sub-A2}  Terrence "Uncle Terry" Richardson (born August 14, 1965) is an American fashion and portrait photographer who has shot advertising campaigns for Marc Jacobs, Aldo, Supreme, Sisley, Tom Ford, and Yves Saint Laurent among others. \\
            \cmidrule(l){1-2}
  \multirow{2}{1cm}{\useqtoseq + FastText}
                 & {\bf Sub-Q1} who is annie morton? \\
                 %& {\bf Sub-A1} Annie Morton (born October 8, 1970) is an American model born in Pennsylvania. \\
                &   {\bf Sub-Q2}  when was terry richardson born? \\
            %& {\bf Sub-A2}  Kenton Terry Richardson (born 26 July 1999) is an English professional footballer who plays as a defender for League Two side Hartlepool United. \\
                \cmidrule(l){1-2}
  \multirow{2}{1cm}{\seqtoseq + Random}
                 & {\bf Sub-Q1} what is the maximum number of students allowed to take part in the program? \\
                 %& {\bf Sub-A1} Kenton Terry Richardson (born 26 July 1999) is an English professional footballer who plays as a defender for League Two side Hartlepool United. \\
                &   {\bf Sub-Q2}  what is the maximum number of students allowed to take part in the program? \\
            %& {\bf Sub-A2} Kenton Terry Richardson (born 26 July 1999) is an English professional footballer who plays as a defender for League Two side Hartlepool United. \\
                \cmidrule(l){1-2}
  \multirow{2}{1cm}{\seqtoseq + FastText}
                 & {\bf Sub-Q1} who is terry morton? \\
                 %& {\bf Sub-A1} Terrence "Uncle Terry" Richardson (born August 14, 1965) is an American fashion and portrait photographer who has shot advertising campaigns for Marc Jacobs, Aldo, Supreme, Sisley, Tom Ford, and Yves Saint Laurent among others. \\
                &   {\bf Sub-Q2}  who is terry morton? \\
            %& {\bf Sub-A2} Terrence "Uncle Terry" Richardson (born August 14, 1965) is an American fashion and portrait photographer who has shot advertising campaigns for Marc Jacobs, Aldo, Supreme, Sisley, Tom Ford, and Yves Saint Laurent among others. \\
                \cmidrule(l){1-2}
  \multirow{2}{1cm}{PseudoD + Random}
                 & {\bf Sub-Q1} what did decnet phase i become? \\
                 %& {\bf Sub-A1} Snoecks is a Belgian magazine. The huge, 550-plus-page magazine appears once a year in October and focuses on the most interesting new international developments in the arts, photography and literature. \\
                &   {\bf Sub-Q2}  what group can amend the victorian constitution? \\
            %& {\bf Sub-A2} Kenton Terry Richardson (born 26 July 1999) is an English professional footballer who plays as a defender for League Two side Hartlepool United. \\
                \cmidrule(l){1-2}
  \multirow{2}{1cm}{PseudoD + FastText}
                 & {\bf Sub-Q1} who was terry richardson? \\
                 %& {\bf Sub-A1} Terrence "Uncle Terry" Richardson (born August 14, 1965) is an American fashion and portrait photographer who has shot advertising campaigns for Marc Jacobs, Aldo, Supreme, Sisley, Tom Ford, and Yves Saint Laurent among others. \\
                &   {\bf Sub-Q2}  who changes positions more , annie morton , cotton hill , or terry richardson? \\
            %& {\bf Sub-A2} Annie Morton (born October 8, 1970) is an American model born in Pennsylvania. \\
                \cmidrule(l){1-2}
  \multirow{2}{1cm}{DecompRC}
                 & {\bf Sub-Q1} annie morton is born when? \\
                 %& {\bf Sub-A1} Annie Morton (born October 8, 1970) is an American model born in Pennsylvania. \\
                &   {\bf Sub-Q2}  terry richardson is born when? \\
            %& {\bf Sub-A2} Terrence "Uncle Terry" Richardson (born August 14, 1965) is an American fashion and portrait photographer who has shot advertising campaigns for Marc Jacobs, Aldo, Supreme, Sisley, Tom Ford, and Yves Saint Laurent among others. \\
                \cmidrule(l){1-2}
  \multirow{2}{1cm}{Variable \useqtoseq + FastText}
            & {\bf Sub-Q1} who is annie morton? \\
            % & {\bf Sub-A1} annie morton (born october 8, 1970) is an american model born in pennsylvania. \\
            &  {\bf Sub-Q2}  who was terry morton? \\
            %& {\bf Sub-A2} madonna is a biography by english author andrew morton, chronicling the life of american recording artist madonna. \\
        \bottomrule
    \end{tabular}
    % }
    \vskip -0.7em
    \caption{Various decomposition methods for the question ``Who is older, Annie Morton or Terry Richardson?"}
    \label{tab:appendix_decomp_examples_2}
    \end{table*}            
            
            \begin{table*}[th!]
    \centering
    \scriptsize
    % \scalebox{0.9}{
    \begin{tabular}{p{1.2cm}p{15cm}}        \toprule

\multicolumn{2}{c}{  {\bf Q:} In which year was the King who made the 1925 Birthday Honours born?} \\ \midrule \multirow{2}{1cm}{\useqtoseq + Random}
            & {\bf Sub-Q1} in which year was the king made? \\
             %& {\bf Sub-A1} George V (George Frederick Ernest Albert; 3 June 1865 – 20 January 1936) was King of the United Kingdom and the British Dominions, and Emperor of India, from 6 May 1910 until his death in 1936. \\
            &  {\bf Sub-Q2}  who made the 1925 birthday honours? \\
            %& {\bf Sub-A2} The 1925 Birthday Honours were appointments by King George V to various orders and honours to reward and highlight good works by citizens of the British Empire. \\
            \cmidrule(l){1-2}
  \multirow{2}{1cm}{\useqtoseq + FastText}
                 & {\bf Sub-Q1} in which year was the king born? \\
                 %& {\bf Sub-A1} George V (George Frederick Ernest Albert; 3 June 1865 – 20 January 1936) was King of the United Kingdom and the British Dominions, and Emperor of India, from 6 May 1910 until his death in 1936. \\
                &   {\bf Sub-Q2}  who made the 1925 birthday honours? \\
            %& {\bf Sub-A2} The 1925 Birthday Honours were appointments by King George V to various orders and honours to reward and highlight good works by citizens of the British Empire. \\
                \cmidrule(l){1-2}
  \multirow{2}{1cm}{\seqtoseq + Random}
                 & {\bf Sub-Q1} what is the maximum number of students allowed to take part in the program? \\
                 %& {\bf Sub-A1} George V (George Frederick Ernest Albert; 3 June 1865 – 20 January 1936) was King of the United Kingdom and the British Dominions, and Emperor of India, from 6 May 1910 until his death in 1936. \\
                &   {\bf Sub-Q2}  what is the maximum number of students allowed to take part in the course of the course of the course of the course of the course of the course of the course of the course of the course of the course of the course of the course of the course? \\
            %& {\bf Sub-A2} George V (George Frederick Ernest Albert; 3 June 1865 – 20 January 1936) was King of the United Kingdom and the British Dominions, and Emperor of India, from 6 May 1910 until his death in 1936. \\
                \cmidrule(l){1-2}
  \multirow{2}{1cm}{\seqtoseq + FastText}
                 & {\bf Sub-Q1} who was born in 1925? \\
                 %& {\bf Sub-A1} George V (George Frederick Ernest Albert; 3 June 1865 – 20 January 1936) was King of the United Kingdom and the British Dominions, and Emperor of India, from 6 May 1910 until his death in 1936. \\
                &   {\bf Sub-Q2}  in which year was the king born? \\
            %& {\bf Sub-A2} George V (George Frederick Ernest Albert; 3 June 1865 – 20 January 1936) was King of the United Kingdom and the British Dominions, and Emperor of India, from 6 May 1910 until his death in 1936. \\
                \cmidrule(l){1-2}
  \multirow{2}{1cm}{PseudoD + Random}
                 & {\bf Sub-Q1} what did telecom australia start? \\
                 %& {\bf Sub-A1} George V (George Frederick Ernest Albert; 3 June 1865 – 20 January 1936) was King of the United Kingdom and the British Dominions, and Emperor of India, from 6 May 1910 until his death in 1936. \\
                &   {\bf Sub-Q2}  what cells are not eliminated by the immune system? \\
            %& {\bf Sub-A2} George V (George Frederick Ernest Albert; 3 June 1865 – 20 January 1936) was King of the United Kingdom and the British Dominions, and Emperor of India, from 6 May 1910 until his death in 1936. \\
                \cmidrule(l){1-2}
  \multirow{2}{1cm}{PseudoD + FastText}
                 & {\bf Sub-Q1} in the new year honours list , who was awarded the mbe for services to hockey? \\
                 %& {\bf Sub-A1} George V (George Frederick Ernest Albert; 3 June 1865 – 20 January 1936) was King of the United Kingdom and the British Dominions, and Emperor of India, from 6 May 1910 until his death in 1936. \\
                &   {\bf Sub-Q2}  in 1925 when she was born? \\
            %& {\bf Sub-A2} George V (George Frederick Ernest Albert; 3 June 1865 – 20 January 1936) was King of the United Kingdom and the British Dominions, and Emperor of India, from 6 May 1910 until his death in 1936. \\
                \cmidrule(l){1-2}
  \multirow{2}{1cm}{DecompRC}
                 & {\bf Sub-Q1} which king who made the 1925 birthday honours? \\
                 %& {\bf Sub-A1} The 1925 Birthday Honours were appointments by King George V to various orders and honours to reward and highlight good works by citizens of the British Empire. \\
                &   {\bf Sub-Q2}  in which year was george v born? \\
            %& {\bf Sub-A2} George V (George Frederick Ernest Albert; 3 June 1865 – 20 January 1936) was King of the United Kingdom and the British Dominions, and Emperor of India, from 6 May 1910 until his death in 1936. \\
                \cmidrule(l){1-2}
  \multirow{2}{1cm}{Variable \useqtoseq + FastText}
            & {\bf Sub-Q1} in which year was the king made? \\
            &  {\bf Sub-A1} george v (george frederick ernest albert; 3 june 1865 – 20 january 1936) was king of the united kingdom and the british dominions, and emperor of india, from 6 may 1910 until his death in 1936. \\
            &  {\bf Sub-Q2}  who made the 1925 birthday honours? \\
            %& {\bf Sub-A2} george v (george frederick ernest albert; 3 june 1865 – 20 january 1936) was king of the united kingdom and the british dominions, and emperor of india, from 6 may 1910 until his death in 1936. \\
        \bottomrule
    \end{tabular}
    % }
    \vskip -0.7em
    \caption{Various decomposition methods for the question ``In which year was the King who made the 1925 Birthday Honours born?"}
    \label{tab:appendix_decomp_examples_4}
    \end{table*}            
            
\begin{table*}[th!]
    \centering
    \scriptsize
    % \scalebox{0.9}{
    \begin{tabular}{p{1.2cm}p{15cm}}        \toprule

\multicolumn{2}{c}{  {\bf Q:} Where are Teide National Park and Garajonay National Park located?} \\ \midrule \multirow{2}{1cm}{\useqtoseq + Random}
            & {\bf Sub-Q1} where are teide national park? \\
             %& {\bf Sub-A1} Teide National Park (Spanish: "Parque nacional del Teide") is a national park located in Tenerife (Canary Islands, Spain). \\
            &  {\bf Sub-Q2}  what is garajonay national park? \\
            %& {\bf Sub-A2} Garajonay National Park (Spanish: "Parque nacional de Garajonay") is located in the center and north of the island of La Gomera, one of the Canary Islands (Spain). It was declared a national park in 1981 and a World Heritage Site by UNESCO in 1986. \\
            \cmidrule(l){1-2}
  \multirow{2}{1cm}{\useqtoseq + FastText}
                 & {\bf Sub-Q1} where are teide national park? \\
                 %& {\bf Sub-A1} Teide National Park (Spanish: "Parque nacional del Teide") is a national park located in Tenerife (Canary Islands, Spain). \\
                &   {\bf Sub-Q2}  where is garajonay national park? \\
            %& {\bf Sub-A2} Garajonay National Park (Spanish: "Parque nacional de Garajonay") is located in the center and north of the island of La Gomera, one of the Canary Islands (Spain). It was declared a national park in 1981 and a World Heritage Site by UNESCO in 1986. \\
                \cmidrule(l){1-2}
  \multirow{2}{1cm}{\seqtoseq + Random}
                 & {\bf Sub-Q1} what is the maximum number of students allowed to take part in the program? \\
                 %& {\bf Sub-A1} Teide National Park (Spanish: "Parque nacional del Teide") is a national park located in Tenerife (Canary Islands, Spain). \\
                &   {\bf Sub-Q2}  what is the maximum number of students allowed to take part in the course of the course of the course of the course of the course of the course of the course of the course of the course of the course of the course of the course of the course? \\
            %& {\bf Sub-A2} It occupies 40 km (15 sq mi) and it extends into each of the six municipalities on the island. \\
                \cmidrule(l){1-2}
  \multirow{2}{1cm}{\seqtoseq + FastText}
                 & {\bf Sub-Q1} where is garajonay national park located? \\
                 %& {\bf Sub-A1} Garajonay National Park (Spanish: "Parque nacional de Garajonay") is located in the center and north of the island of La Gomera, one of the Canary Islands (Spain). It was declared a national park in 1981 and a World Heritage Site by UNESCO in 1986. \\
                &   {\bf Sub-Q2}  the national park of galicia national park? \\
            %& {\bf Sub-A2} Teide National Park (Spanish: "Parque nacional del Teide") is a national park located in Tenerife (Canary Islands, Spain). \\
                \cmidrule(l){1-2}
  \multirow{2}{1cm}{PseudoD + Random}
                 & {\bf Sub-Q1} what was the australian public x.75 network operated by telstra? \\
                 %& {\bf Sub-A1} Teide National Park (Spanish: "Parque nacional del Teide") is a national park located in Tenerife (Canary Islands, Spain). \\
                &   {\bf Sub-Q2}  when were theories developed suggesting inequality may have some positive effect on economic development? \\
            %& {\bf Sub-A2} Teide National Park (Spanish: "Parque nacional del Teide") is a national park located in Tenerife (Canary Islands, Spain). \\
                \cmidrule(l){1-2}
  \multirow{2}{1cm}{PseudoD + FastText}
                 & {\bf Sub-Q1} where is garajonay national park? \\
                 %& {\bf Sub-A1} Garajonay National Park (Spanish: "Parque nacional de Garajonay") is located in the center and north of the island of La Gomera, one of the Canary Islands (Spain). It was declared a national park in 1981 and a World Heritage Site by UNESCO in 1986. \\
                &   {\bf Sub-Q2}  how to visit the teide observatory in tenerife in what languages are guided tours of the teide observatory held? \\
            %& {\bf Sub-A2} Teide National Park (Spanish: "Parque nacional del Teide") is a national park located in Tenerife (Canary Islands, Spain). \\
                \cmidrule(l){1-2}
  \multirow{2}{1cm}{DecompRC}
                 & {\bf Sub-Q1} where is teide national park located? \\
                 %& {\bf Sub-A1} Teide National Park (Spanish: "Parque nacional del Teide") is a national park located in Tenerife (Canary Islands, Spain). \\
                &   {\bf Sub-Q2}  where is garajonay national park located? \\
            %& {\bf Sub-A2} Garajonay National Park (Spanish: "Parque nacional de Garajonay") is located in the center and north of the island of La Gomera, one of the Canary Islands (Spain). It was declared a national park in 1981 and a World Heritage Site by UNESCO in 1986. \\
                \cmidrule(l){1-2}
  \multirow{2}{1cm}{Variable \useqtoseq + FastText}
            & {\bf Sub-Q1} where are teide national park? \\
            &  {\bf Sub-A1} teide national park (spanish: "parque nacional del teide") is a national park located in tenerife (canary islands, spain). \\
            &  {\bf Sub-Q2}  where is garajonay national park? \\
            %& {\bf Sub-A2} garajonay national park (spanish: "parque nacional de garajonay") is located in the center and north of the island of la gomera, one of the canary islands (spain). \\
        \bottomrule
    \end{tabular}
    % }
    \vskip -0.7em
    \caption{Various decomposition methods for the question ``Where are Teide National Park and Garajonay National Park located?}
    \label{tab:appendix_decomp_examples_5}
    \end{table*}            
            
    %\end{table*}            
            
            \begin{table*}[th!]
    \centering
    \scriptsize
    % \scalebox{0.9}{
    \begin{tabular}{p{1.2cm}p{15cm}}        \toprule

    \multicolumn{2}{c}{  {\bf Q:} Since 2 June 2017, The Leader of Fine Gael had been held by which Irish Fine Gael politician who has served as Taoiseach and Minister for Defence?} \\ \midrule \multirow{2}{1cm}{\useqtoseq + Random}
            & {\bf Sub-Q1} how long since 2 june 2017 , the leader of fine gael had been in office? \\
             %& {\bf Sub-A1} Enda Patrick Kenny (born 24 April 1951) is an Irish Fine Gael politician who served as Taoiseach from 2011 to 2017, Leader of Fine Gael from 2002 to 2017, Minister for Defence from May 2014 to July 2014 and 2016 to 2017, Leader of the Opposition from 2002 to 2011, Minister for Tourism and Trade from 1994 to 1997 and Minister of State for Youth Affairs from 1986 to 1987. \\
            &  {\bf Sub-Q2}  which irish fine gael politician has served as taoiseach and minister for defence? \\
            %& {\bf Sub-A2} Leo Eric Varadkar ( ; Irish: "Leo de Varad" ;born 18 January 1979) is an Irish Fine Gael politician who has served as Taoiseach, Minister for Defence and Leader of Fine Gael since June 2017. \\
            \cmidrule(l){1-2}
  \multirow{2}{1cm}{\useqtoseq + FastText}
                 & {\bf Sub-Q1} since 2 june 2017 , the leader of fine gael had been? \\
                 %& {\bf Sub-A1} Since 2 June 2017, the office had been held by Leo Varadkar following the resignation of Enda Kenny. \\
                &   {\bf Sub-Q2}  which irish fine gael politician has served as taoiseach and minister for defence? \\
            %& {\bf Sub-A2} Leo Eric Varadkar ( ; Irish: "Leo de Varad" ;born 18 January 1979) is an Irish Fine Gael politician who has served as Taoiseach, Minister for Defence and Leader of Fine Gael since June 2017. \\
                \cmidrule(l){1-2}
  \multirow{2}{1cm}{\seqtoseq + Random}
                 & {\bf Sub-Q1} what is the maximum number of students allowed to take part in the program? \\
                 %& {\bf Sub-A1} Leo Eric Varadkar ( ; Irish: "Leo de Varad" ;born 18 January 1979) is an Irish Fine Gael politician who has served as Taoiseach, Minister for Defence and Leader of Fine Gael since June 2017. \\
                &   {\bf Sub-Q2}  what is the maximum number of students allowed per year? \\
            %& {\bf Sub-A2} The Leader of Fine Gael is the most senior politician within the Fine Gael political party in Ireland. Since 2 June 2017, the office had been held by Leo Varadkar following the resignation of Enda Kenny. \\
                \cmidrule(l){1-2}
  \multirow{2}{1cm}{\seqtoseq + FastText}
                 & {\bf Sub-Q1} who has been appointed as the new deputy leader of fine gael since 2 june 2017? \\
                 %& {\bf Sub-A1} Simon Anthony Coveney (born 16 June 1972) is an Irish Fine Gael politician who has served as Minister for Foreign Affairs and Trade and Deputy Leader of Fine Gael since June 2017. \\
                &   {\bf Sub-Q2}  the fine gael fine gael , the fine gael of fine gael? \\
            %& {\bf Sub-A2} Leo Eric Varadkar ( ; Irish: "Leo de Varad" ;born 18 January 1979) is an Irish Fine Gael politician who has served as Taoiseach, Minister for Defence and Leader of Fine Gael since June 2017. \\
                \cmidrule(l){1-2}
  \multirow{2}{1cm}{PseudoD + Random}
                 & {\bf Sub-Q1} what was considered to be a major milestone? \\
                 %& {\bf Sub-A1} The 2017 Fine Gael leadership election was triggered in May 2017, when Enda Kenny resigned as party leader. \\
                &   {\bf Sub-Q2}  what was the air force not interested in for their message system? \\
            %& {\bf Sub-A2} The 2017 Fine Gael leadership election was triggered in May 2017, when Enda Kenny resigned as party leader. \\
                \cmidrule(l){1-2}
  \multirow{2}{1cm}{PseudoD + FastText}
                 & {\bf Sub-Q1} what if fine gael did support fine gael after the next election? \\
                 %& {\bf Sub-A1} With Fine Gael being the governing party at the time, this election effectively appointed a new Taoiseach for Ireland. \\
                &   {\bf Sub-Q2}  who has been appointed as defence minister of india? \\
            %& {\bf Sub-A2} Leo Eric Varadkar ( ; Irish: "Leo de Varad" ;born 18 January 1979) is an Irish Fine Gael politician who has served as Taoiseach, Minister for Defence and Leader of Fine Gael since June 2017. \\
                \cmidrule(l){1-2}
  \multirow{2}{1cm}{DecompRC}
                 & {\bf Sub-Q1} which leader of fine gael? \\
                 %& {\bf Sub-A1} Since 2 June 2017, the office had been held by Leo Varadkar following the resignation of Enda Kenny. \\
                &   {\bf Sub-Q2}  since 2 june 2017 enda patrick kenny had been held by which irish fine gael politician who has served as taoiseach and minister for defence? \\
            %& {\bf Sub-A2} Leo Eric Varadkar ( ; Irish: "Leo de Varad" ;born 18 January 1979) is an Irish Fine Gael politician who has served as Taoiseach, Minister for Defence and Leader of Fine Gael since June 2017. \\
                \cmidrule(l){1-2}
  \multirow{2}{1cm}{Variable \useqtoseq + FastText}
            & {\bf Sub-Q1} since 2 june 2017 , the leader of fine gael had been held by? \\
            % &  {\bf Sub-A1} since 2 june 2017, the office had been held by leo varadkar following the resignation of enda kenny. \\
            &  {\bf Sub-Q2}  which irish fine gael politician has served as taoiseach and minister for defence? \\
            %& {\bf Sub-A2} enda patrick kenny (born 24 april 1951) is an irish fine gael politician who served as taoiseach from 2011 to 2017, leader of fine gael from 2002 to 2017, minister for defence from may 2014 to july 2014 and 2016 to 2017, leader of the opposition from 2002 to 2011, minister for tourism and trade from 1994 to 1997 and minister of state for youth affairs from 1986 to 1987. he has been a teachta dála (td) since 1975, currently for the mayo constituency. \\

        \bottomrule
    \end{tabular}
    % }
    \vskip -0.7em
    \caption{Various decomposition methods for the question ``Since 2 June 2017, The Leader of Fine Gael had been held by which Irish Fine Gael politician who has served as Taoiseach and Minister for Defence?"}
    \label{tab:appendix_decomp_examples_6}
    \end{table*}
